# Supplementary material for: Learning Sample Reweighting for Accuracy and Adversarial Robustness
Source: arXiv:2210.11513 source file (2022-10-20)
Supplement: Supplementary file 1 [file appendix_bu.tex]

\section{Appendix}

\subsection{Derivation of Meta Gradient}
In this section we give the derivation of Eq. \ref{eq:wupdate}:
\begin{equation}
\frac{\partial \hat{\mathcal{L}}_{\textrm{val}}(\theta_t)}{\partial w_i} = -\frac{\alpha}{m_\textrm{val}}\sum_{j}^{m_{\textrm{val}}}\left(\nabla_{\theta} \hat{\ell}_{\textrm{val}}(\theta_t)\right)^T\nabla_{\theta} \hat{\ell}_{\textrm{tr}}(\theta_{t-1})
\label{eq:wupdateapdx}
\end{equation}
We are interested in finding $\frac{\partial \hat{\mathcal{L}}_{\textrm{val}}(\theta_t)}{\partial w_i}$-- the update for example weight $i$. Let 
$$\hat{\mathcal{L}}_{\textrm{tr}}(\theta_t, w) = \frac{1}{m_{\textrm{tr}}}\sum_{i=1}^{m_{\textrm{tr}}}w_i\hat{\ell}_i(\theta_t)$$ be the robust training loss with respect to parameters $\theta$ at time $t$ and example weight $w_i$ for the $i$-th training example. Let $\hat{\mathcal{L}}_{\textrm{val}}(\theta_t) = \frac{1}{m_{\textrm{val}}}\sum_{i=1}^{m_{\textrm{val}}}\hat{\ell}_i(\theta_t)$ be the associated \textit{unweighted} validation loss. Following the meta-learning framework, we to minimize this loss.

We are interested in finding $\frac{\partial \hat{\mathcal{L}}_{\textrm{val}}(\theta_t)}{\partial w_i}$-- the update for example weight $i$.
\begin{align*}
\frac{\partial \hat{\mathcal{L}}_{\textrm{val}}(\theta_t)}{\partial w_i} &= \frac{1}{m_{\textrm{val}}}\sum_{j}^{m_{\textrm{val}}}\frac{\partial \hat{\ell}_{\textrm{val},j}(\theta_t)}{\partial w_i} \\
&= \frac{1}{m_{\textrm{val}}}\sum_{j}^{m_{\textrm{val}}}\left(\nabla_{\theta} \hat{\ell}_{\textrm{val},j}(\theta_{t})\right)^T\frac{\partial \theta_t}{\partial w_i}  \\
\frac{\partial \theta_{t}}{\partial w_i} &= \frac{\partial}{\partial w_i} (\theta_{t-1} - \alpha\nabla_{\theta}\hat{\mathcal{L}}_{\textrm{tr}}(\theta_{t-1},w_i)) \\
&= -\alpha \frac{\partial}{\partial w_i} \nabla_{\theta}\hat{\mathcal{L}}_{\textrm{tr}}(\theta_{t-1},w_i)) \\
&= -\frac{\alpha}{m_{tr}} \frac{\partial}{\partial w_i} \sum_{j}^{m_{\textrm{tr}}}
w_j\nabla_{\theta}\hat{\ell}_{\textrm{tr},j}(\theta_{t-1}) \\
&= -\frac{\alpha}{m_{tr}} \nabla_\theta\hat{\ell}_{\textrm{tr},i}(\theta_{t-1}) \\
\implies\frac{\partial \hat{\mathcal{L}}_{\textrm{val}}(\theta_t)}{\partial w_i} &= -\frac{\alpha}{m_{\textrm{val}}}\sum_{j}^{m_{\textrm{val}}}\left(\nabla_{\theta_{t}} \hat{\ell}_{\textrm{val},j}(\theta_t)\right)^T\nabla_{\theta} \hat{\ell}_{\textrm{tr},i}(\theta_{t-1})
\end{align*}

\subsection{Main Experiments}

\subsubsection{Architectures}
\input{tables/architectures}

We abbreviate one hidden layer fully connected network with 1024 hidden units with FC1. The tiny-CNN convolutional architecture that we use is identical to that of \cite{KolterWongPolytope17, Croce2020Provable} —consisting of two convolutional layers with $16$ and $32$ filters of size $4 \times 4$ and stride $2$, followed by a fully connected layer with $100$ hidden units. For all experiments we use training and validation batch sizes of $128$ and we train all models for $100$ epochs. Moreover, we use the SGD with a cyclic cosine learning rate schedule with maximmum learning rate of $0.02$. On all datasets (MNIST, F-MNIST, and CIFAR-10) we restrict the input to be in the range $[0, 1]$. On the CIFAR-10 dataset, following \cite{zhang2021geometryaware}, we apply random crops and random mirroring of the images as data augmentation during training. In order to make a comparison to the robust training of \cite{zhang2021geometryaware}, we re-train their publicly available models using their github code\footnote{\url{https://github.com/zjfheart/Geometry-aware-Instance-reweighted-Adversarial-Training}}. We perform adversarial training using the PGD attack of \cite{madry2018towards}. For the $\ell_2$-norm experiments, we used the implementation from \cite{rauber2017foolbox} to perform PGD-based $\ell_2$ attacks. During training, we perform 20 iterations of the PGD attack for all datasets. During evaluation, we use 40 iterations for all datasets. Following \cite{zhang2021geometryaware}, the step size is the perturbation radius divided by $4$.

\subsubsection{Details of state-of-the-art methods}
Given an input label pair $(x, y)$, a neural network parameterized by weights $\theta$, and a ``succesfull'' adversarial example $x_{\textrm{adv}}$ associated with $x$, let $\kappa(x,y;\theta)$ denote the number of PGD steps required to construct $x_{\textrm{adv}}$ such that $c(x) \neq c(x_{\textrm{adv}})$. 

\textbf{Geometry-aware Instance Reweighted Adversarial Training (GAIRAT)\cite{zhang2021geometryaware}.} Given an input label pair $(x,y)$, GAIRAT recovers the associated weight $w$ by computing $\kappa(x,y;\theta)$, and mapping $\kappa(x,y;\theta)$ to $w$ via a \textit{weight assignment function} that is monotonically increasing in $\kappa$. The authors evaluate various choices of the weight assignment function, and select the following heuristic:
$$
w(x,y;\theta) = \frac{1 + \tanh(\lambda + 5 \times (1-2\times \kappa(x,y;\theta)/K))}{2}
$$
where $\kappa(x,y;\theta)/K \in [0,1]$.

\textbf{Weighted Minimax Risk (WMMR)\cite{zeng2020adversarial, Wang2020Improving}.} WMMR works similarly. The weight assignment function is chosen to be an exponential function of the \textit{margin} of $f$ at $x_{\textrm{adv}}$:
$$
w(x,y;\theta) = e^{-\alpha\cdot \textrm{margin}(f_\theta,x_{\textrm{adv}},y)}
$$
where the margin function is chosen to be 
$$
\textrm{margin}(f_\theta, x, y) = p(f_\theta(x) = y) - \max_{t\neq y}(f(x) = t)
$$

\subsubsection{Motivating sample reweighting}

\begin{figure}
    \centering
    Low-weight training samples
    \includegraphics[width=\textwidth]{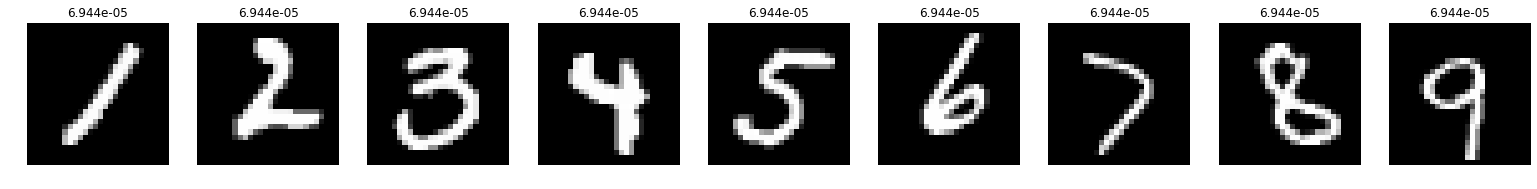}
    \includegraphics[width=\textwidth]{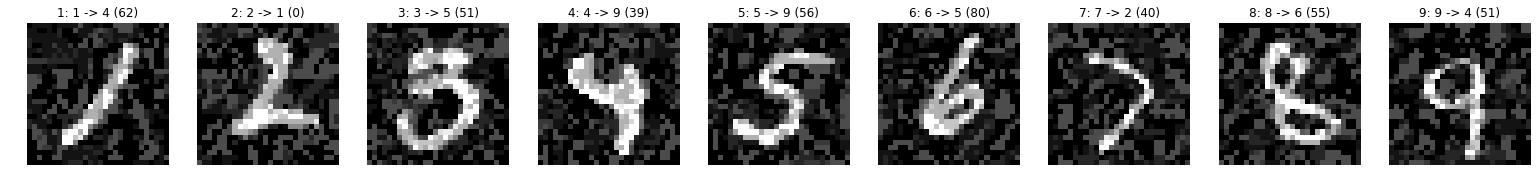}
    
    \vspace{0.5cm}
    High-weight training samples
    \includegraphics[width=\textwidth]{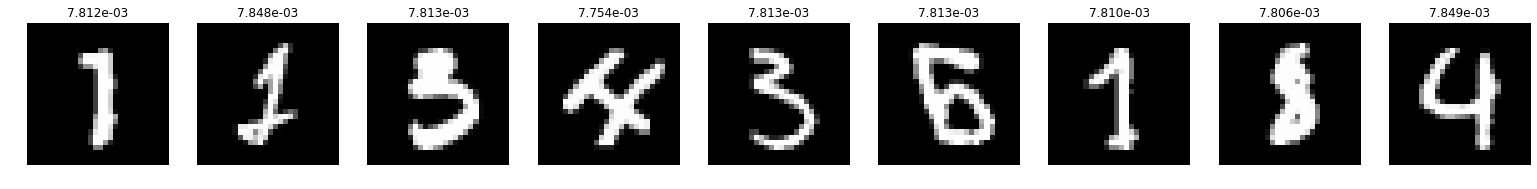}
    \includegraphics[width=\textwidth]{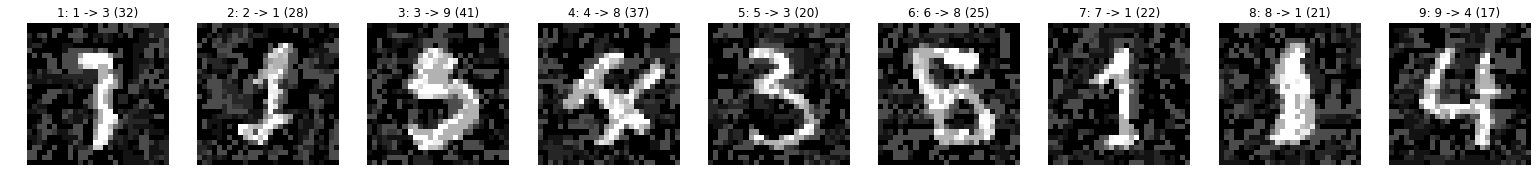}
    \caption{Low weight (top rows) and high weight (bottom rows). Upper rows correspond to clean samples. Bottom rows are adversarial samples generated via PGD. Samples in the upper rows are labeled with weight. Samples in the lower rows are labeled: \textit{true label} : \textit{clean prediction} -> \textit{adversarial prediction} ($\kappa$). Note the ``$5$'' and ``$7$'' (MNIST samples \# $42454$ and \# $25560$).} 
    \label{fig:mnist_examples}
\end{figure}

\begin{figure}
    \centering
    \includegraphics[width=0.85\textwidth]{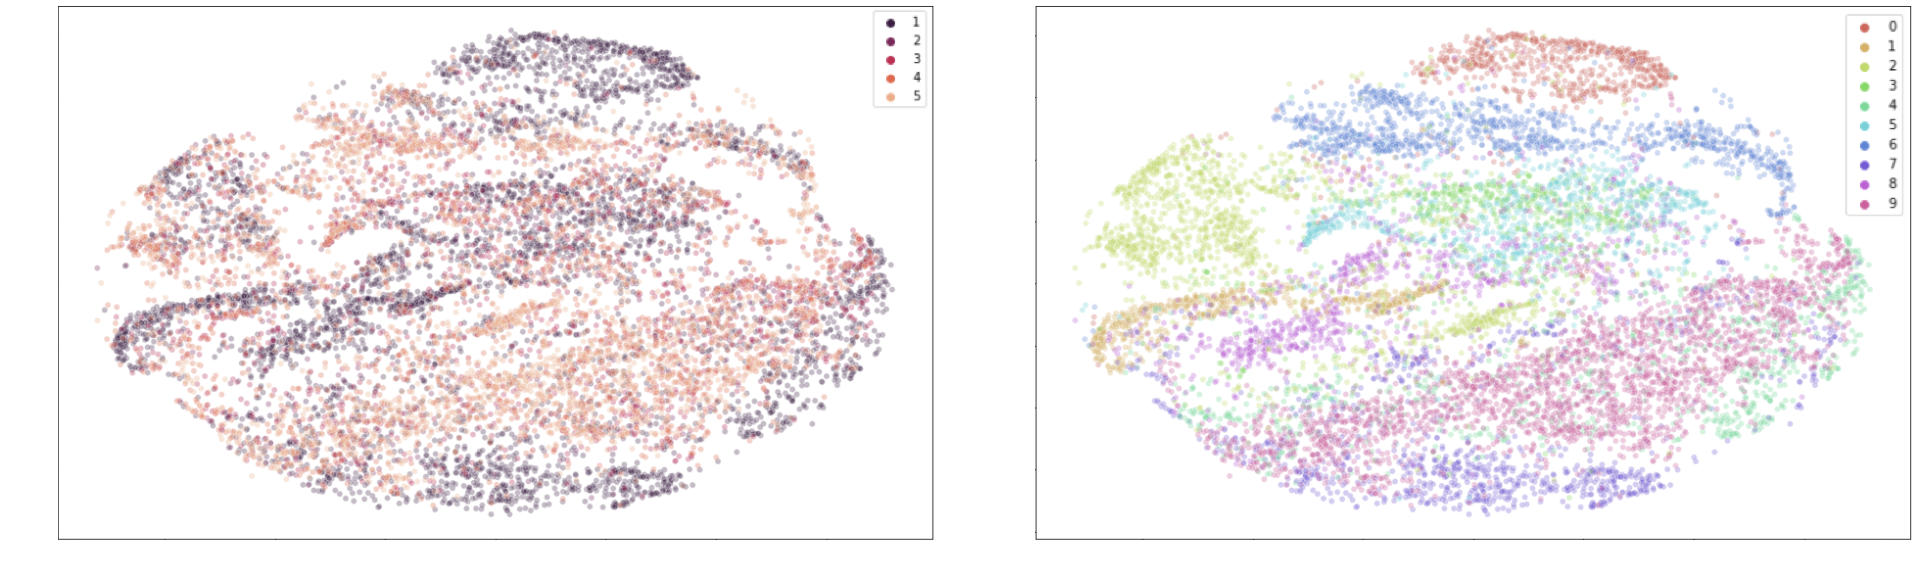}
    \caption{t-SNE plot of MNIST digits. Points in the left-hand plot are colored according to weight (darker samples are high-weight samples, lighter samples are low-weight samples). Points in the right-hand plot are colored according to their label}
    \label{fig:tsne}
\end{figure}

In Fig. \ref{fig:mnist_examples} we identify significant differences in digits that exhibit high weight and low weight. We train a robust SMALL-CNN network on MNIST to high clean and robust-accuracy, and select training samples with largest and smallest weight from each class. In the top two rows, we plot samples with low weights. In the bottom two rows, we plot samples associated with large weights. For both pairs, in the upper row the unnormalized weight is noted above the clean images. In the bottom row of both pairs we plot the corresponding adversarial sample. Above each adversarial example, we write the true label, the prediction made by the network on the clean example, the prediction on the adversarial sample, and the number of PGD steps ($\kappa$)required to switch the label: \textit{true label} : \textit{clean prediction} -> \textit{adversarial prediction} ($\kappa$). $\kappa = 0$ corresponds to a one-step adversarial sample.

In Fig. \ref{fig:tsne} we embed MNIST digits into two dimensions using t-SNE. On the left, samples are colored according to their relative weight. In the right plot samples are colored according to their class. Note that high-weighted samples primarily concentrate in classes (e.g. $0$, $1$, $7$, $3$, $4$). 

In Fig. \ref{fig:weight_distribution}, we plot 2-d visualizations of the output distributions of a robust WRN network on the CIFAR-10 dataset. For each class in the CIFAR-10 dataset, we randomly sample 1000 training datapoints for visualization. For each data point, we compute the least number of iterations $\kappa$ that PGD requires to find its misclassified adversarial variant. For PGD, we set the perturbation bound $\epsilon= 0.031$, the step size $\alpha = 0.31/4$, and the maximum PGD steps $K = 20$. Then, each data point has its unique robustness attribution, i.e., value $\kappa$. We take those data as the input of the robust network and output 10-dimensional logits, and then, we use principal components analysis (PCA) to project 10-dimensional logits into 2-dimension for visualization. The color gradient denotes the degree of the robustness of each data point. Note that the vulnerable samples have lighter colors and are closer to the opposite class, and the more robust samples have darker colors.

From Fig. \ref{fig:weight_distribution}, we find that the vulnerable samples in general are geometrically close to the decision boundary while the samples on which the network is robust in general are far from the boundary. We also note that all classes are well separated. For example, cat-dog and bird-deer are less separable compared to airplane-dog and automobile-horse.

\begin{figure}
\includegraphics[trim={0 0.25cm 0 0},clip,width=0.24\textwidth]{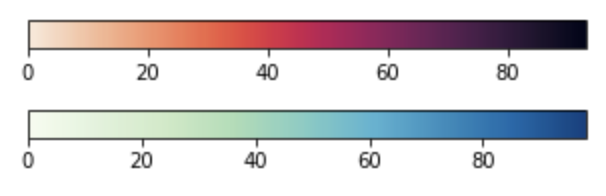}
\includegraphics[width=0.24\textwidth]{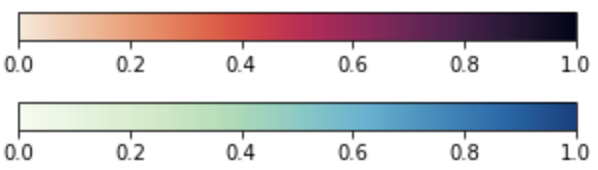}
\includegraphics[trim={0 0.25cm 0 0},clip,width=0.24\textwidth]{figures/pair-plots/scale.png}
\includegraphics[width=0.24\textwidth]{figures/pair-plots-w/scale.png}

\includegraphics[width=0.24\linewidth]{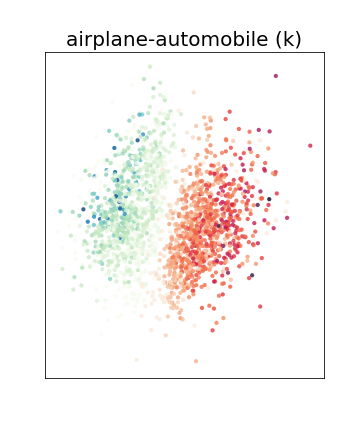}
\includegraphics[width=0.24\linewidth]{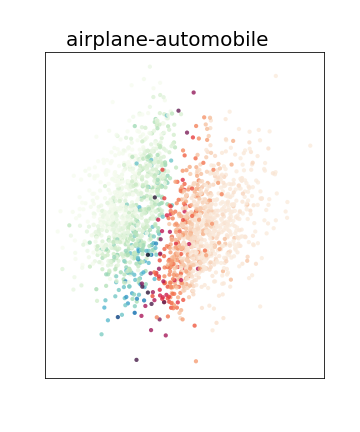}
\includegraphics[width=0.24\linewidth]{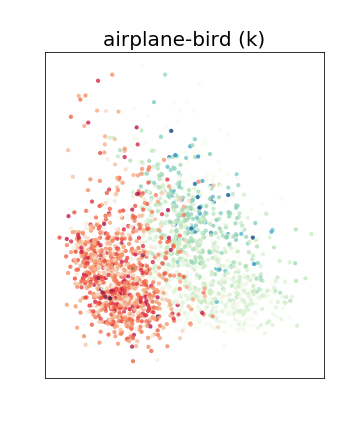}
\includegraphics[width=0.24\linewidth]{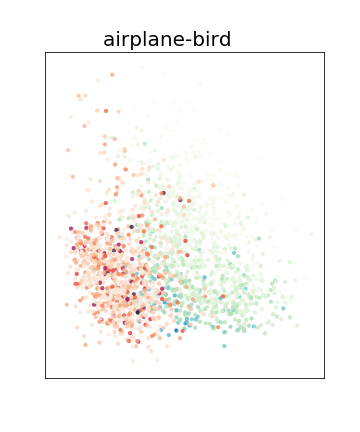}

\vspace{-0.5cm}

\includegraphics[width=0.24\linewidth]{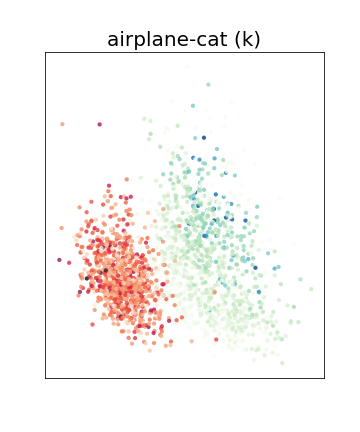}
\includegraphics[width=0.24\linewidth]{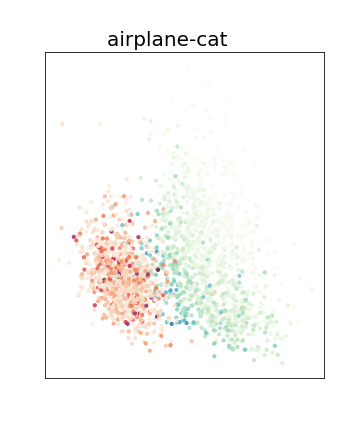}
\includegraphics[width=0.24\linewidth]{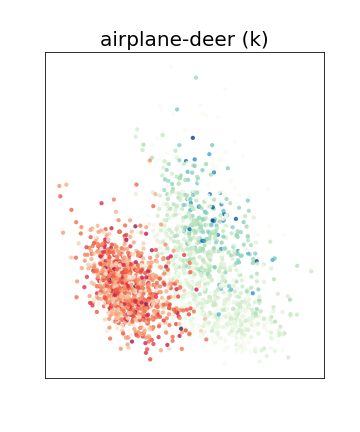}
\includegraphics[width=0.24\linewidth]{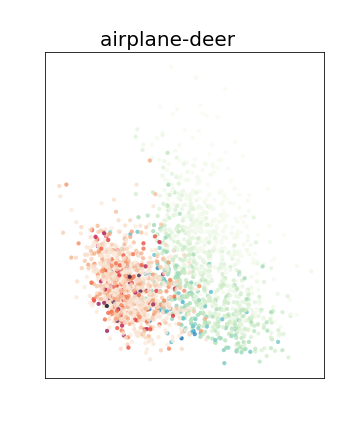}

\vspace{-0.5cm}

\includegraphics[width=0.24\linewidth]{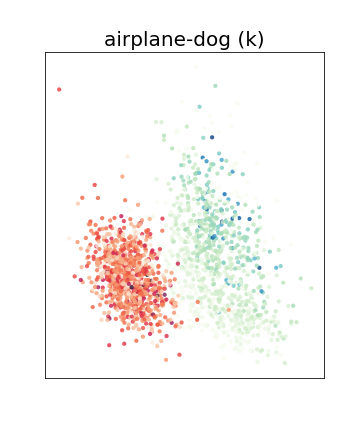}
\includegraphics[width=0.24\linewidth]{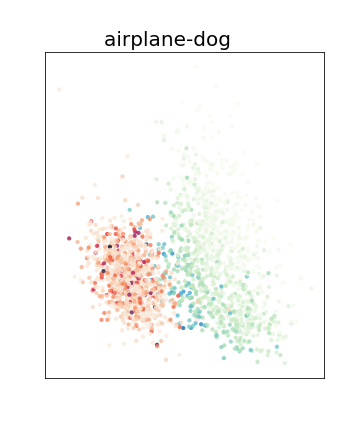}
\includegraphics[width=0.24\linewidth]{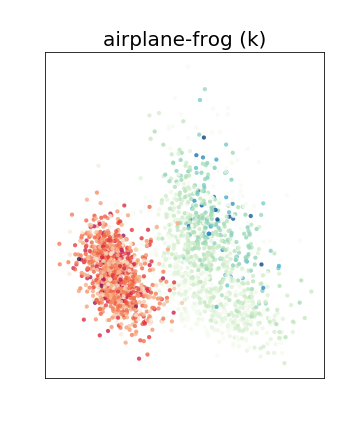}
\includegraphics[width=0.24\linewidth]{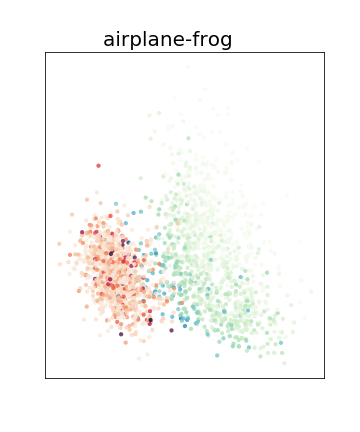}

\vspace{-0.5cm}

\includegraphics[width=0.24\linewidth]{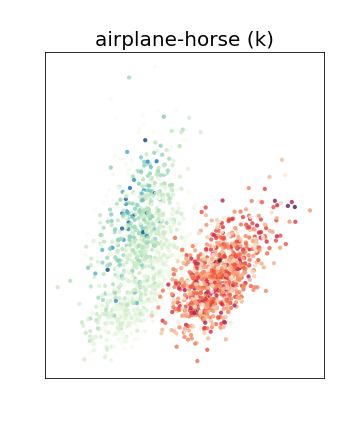}
\includegraphics[width=0.24\linewidth]{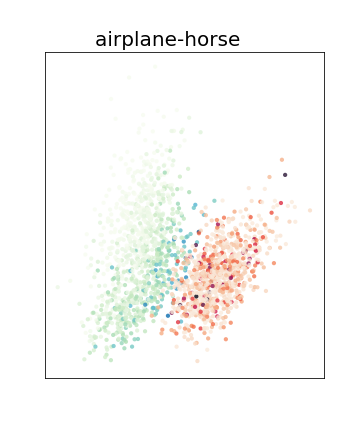}
\includegraphics[width=0.24\linewidth]{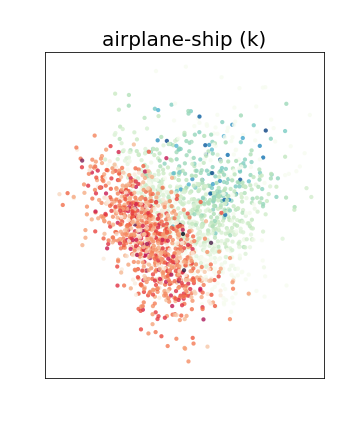}
\includegraphics[width=0.24\linewidth]{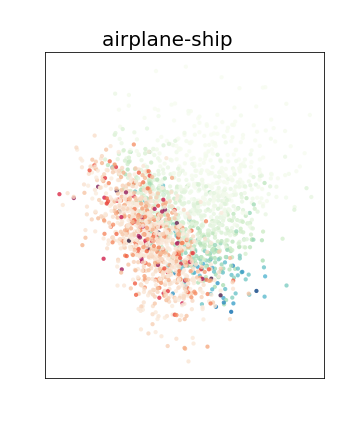}

\vspace{-0.5cm}

\includegraphics[width=0.24\linewidth]{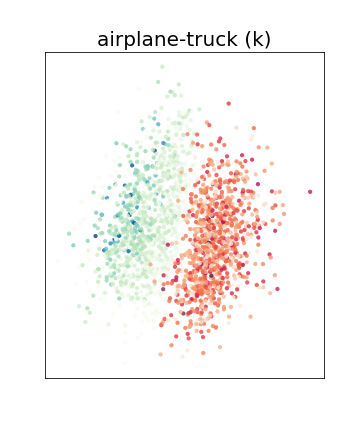}
\includegraphics[width=0.24\linewidth]{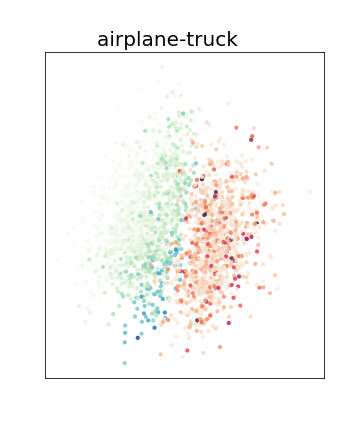}
\includegraphics[width=0.24\linewidth]{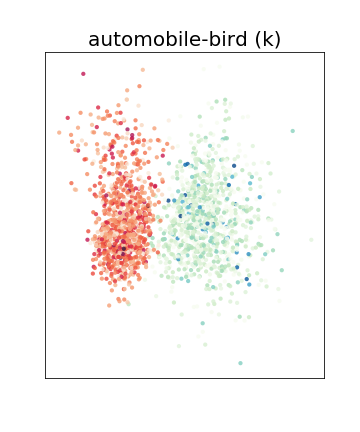}
\includegraphics[width=0.24\linewidth]{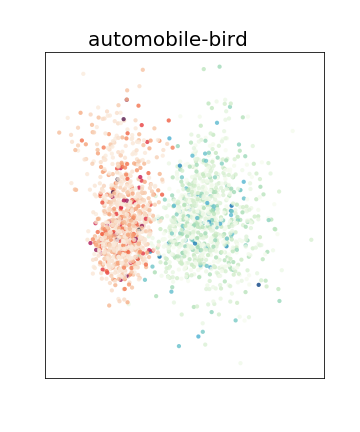}
%%%%%
\caption{\textbf{Part A} 2-d visualizations of the model’s output distribution of natural training data from two separated classes from CIFAR-10 dataset. The weight of a datum corresponds to the intesnity. of the color. The dark blue and dark red points represent samples with higher weight which are close to the class boundary; the light blue and light red points represent the samples with smaller weight. (Top colorbars corresponds to the $0-1$ normalized weights)}
\label{fig:weight_distribution}
\end{figure}

%%%%%%%%

\begin{figure}
\includegraphics[trim={0 0.25cm 0 0},clip,width=0.24\textwidth]{figures/pair-plots/scale.png}
\includegraphics[width=0.24\textwidth]{figures/pair-plots-w/scale.png}
\includegraphics[trim={0 0.25cm 0 0},clip,width=0.24\textwidth]{figures/pair-plots/scale.png}
\includegraphics[width=0.24\textwidth]{figures/pair-plots-w/scale.png}

\includegraphics[width=0.24\linewidth]{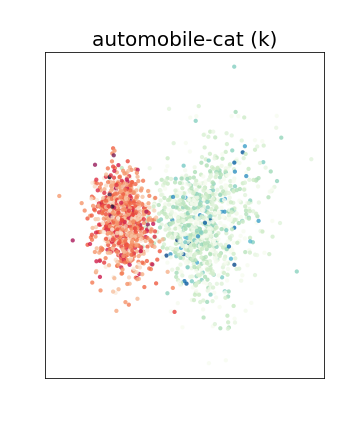}
\includegraphics[width=0.24\linewidth]{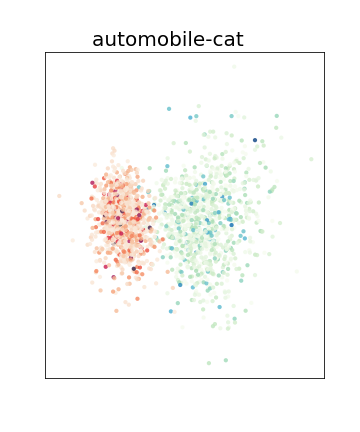}
\includegraphics[width=0.24\linewidth]{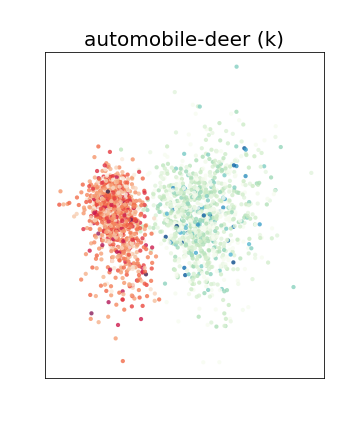}
\includegraphics[width=0.24\linewidth]{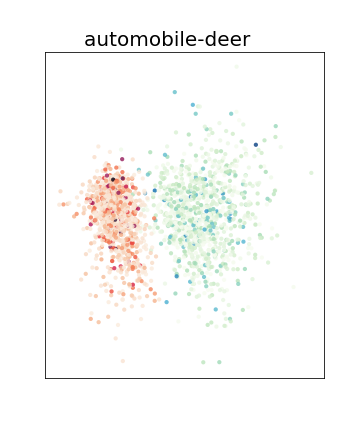}

\vspace{-0.5cm}

\includegraphics[width=0.24\linewidth]{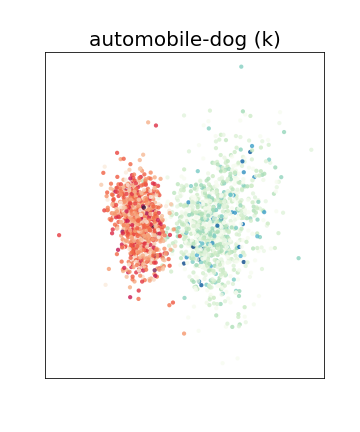}
\includegraphics[width=0.24\linewidth]{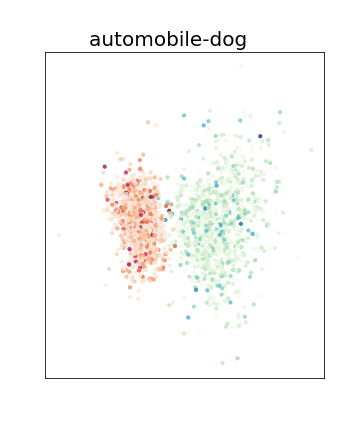}
\includegraphics[width=0.24\linewidth]{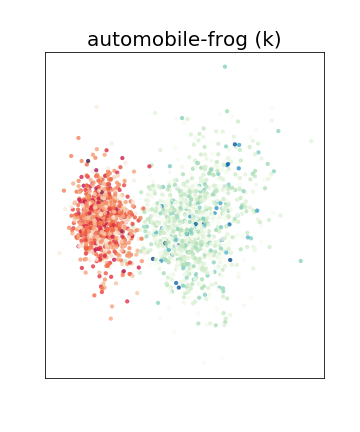}
\includegraphics[width=0.24\linewidth]{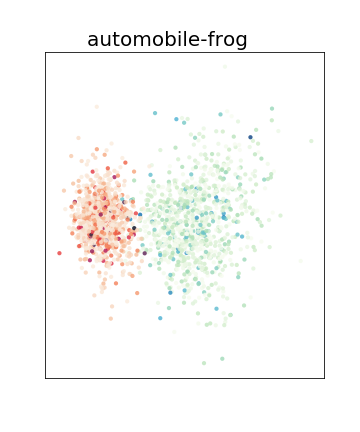}

\vspace{-0.5cm}

\includegraphics[width=0.24\linewidth]{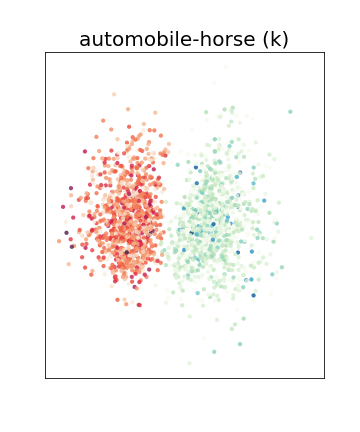}
\includegraphics[width=0.24\linewidth]{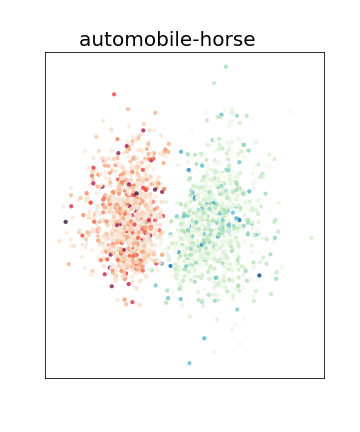}
\includegraphics[width=0.24\linewidth]{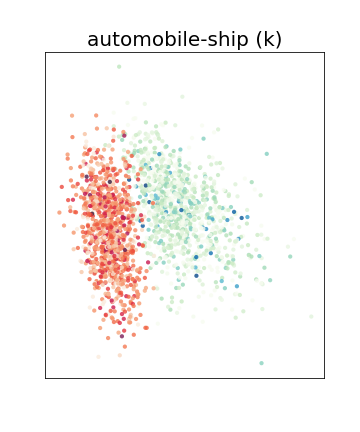}
\includegraphics[width=0.24\linewidth]{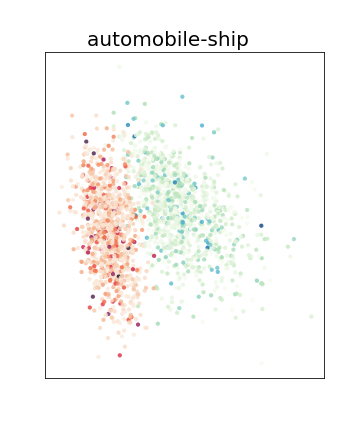}

\vspace{-0.5cm}

\includegraphics[width=0.24\linewidth]{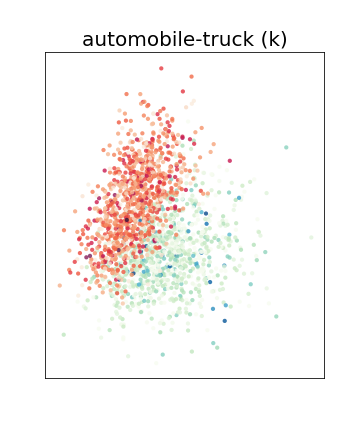}
\includegraphics[width=0.24\linewidth]{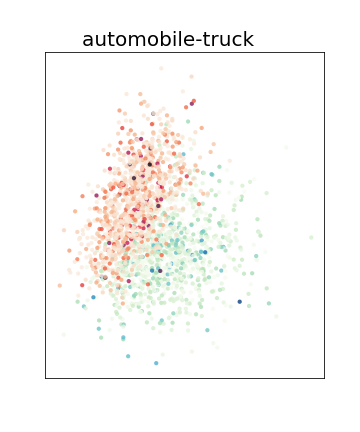}
\includegraphics[width=0.24\linewidth]{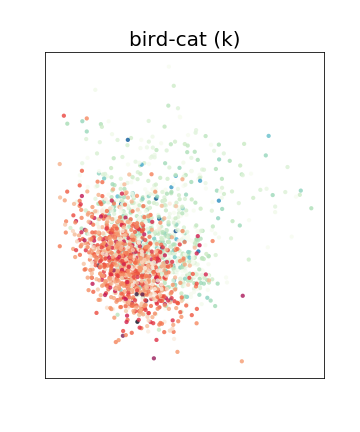}
\includegraphics[width=0.24\linewidth]{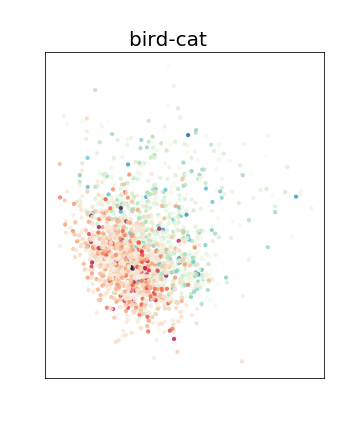}

\vspace{-0.5cm}

\includegraphics[width=0.24\linewidth]{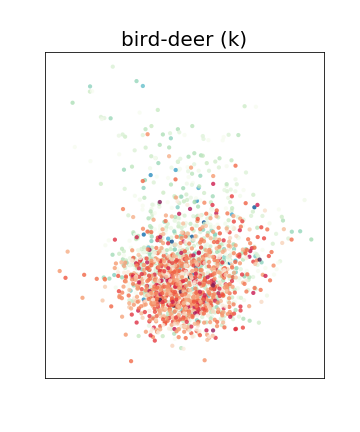}
\includegraphics[width=0.24\linewidth]{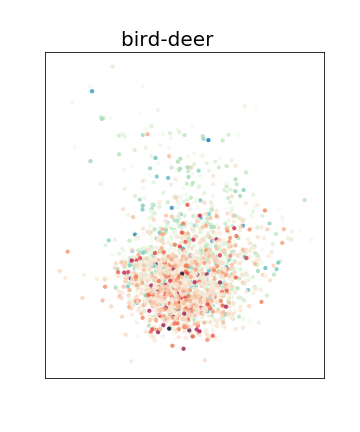}
\includegraphics[width=0.24\linewidth]{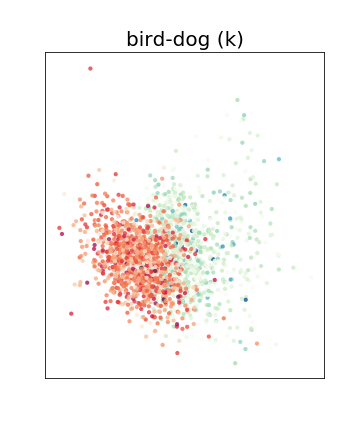}
\includegraphics[width=0.24\linewidth]{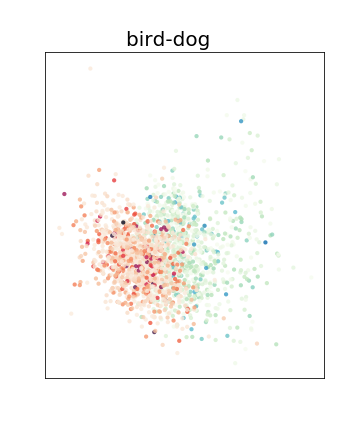}

\vspace{-0.5cm}

\includegraphics[width=0.24\linewidth]{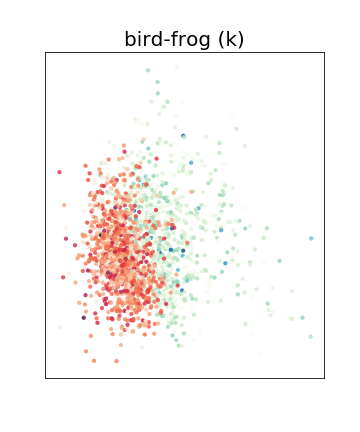}
\includegraphics[width=0.24\linewidth]{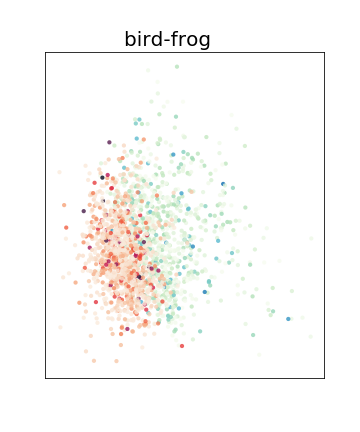}
\includegraphics[width=0.24\linewidth]{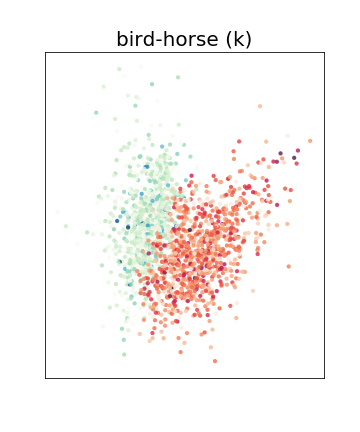}
\includegraphics[width=0.24\linewidth]{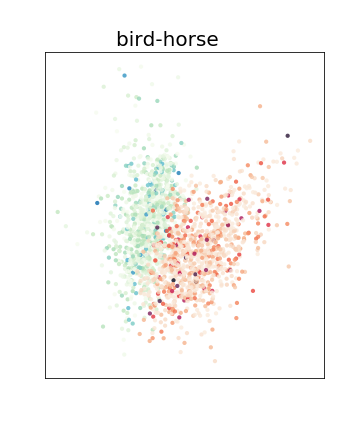}
\caption{\textbf{Part B} 2-d visualizations of the model’s output distribution on CIFAR-10 dataset.}
\end{figure}

%%%%%%%%

\begin{figure}
\includegraphics[trim={0 0.25cm 0 0},clip,width=0.24\textwidth]{figures/pair-plots/scale.png}
\includegraphics[width=0.24\textwidth]{figures/pair-plots-w/scale.png}
\includegraphics[trim={0 0.25cm 0 0},clip,width=0.24\textwidth]{figures/pair-plots/scale.png}
\includegraphics[width=0.24\textwidth]{figures/pair-plots-w/scale.png}

\includegraphics[width=0.24\linewidth]{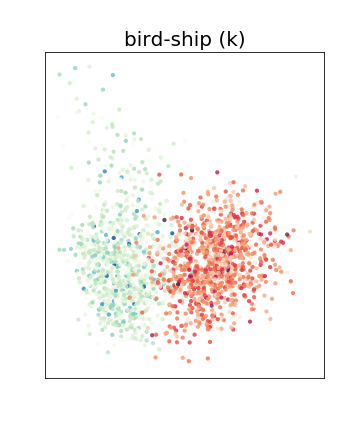}
\includegraphics[width=0.24\linewidth]{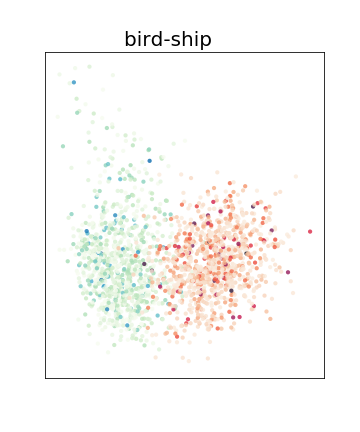}
\includegraphics[width=0.24\linewidth]{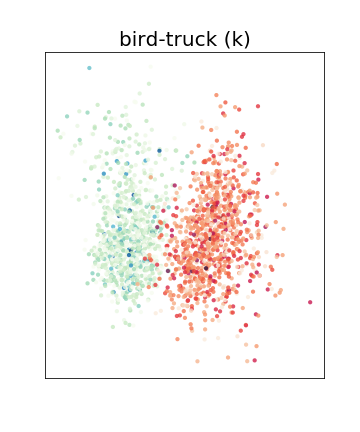}
\includegraphics[width=0.24\linewidth]{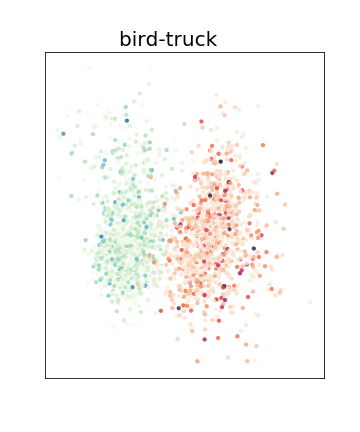}

\vspace{-0.5cm}

\includegraphics[width=0.24\linewidth]{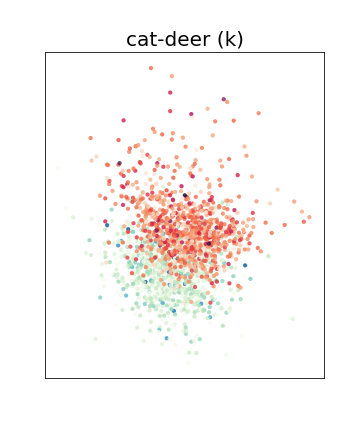}
\includegraphics[width=0.24\linewidth]{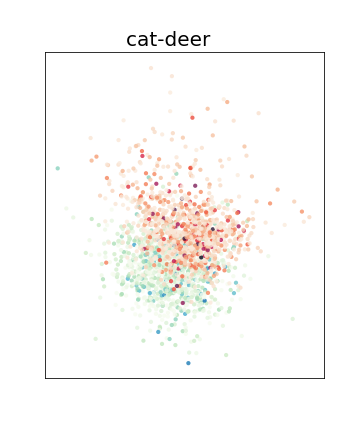}
\includegraphics[width=0.24\linewidth]{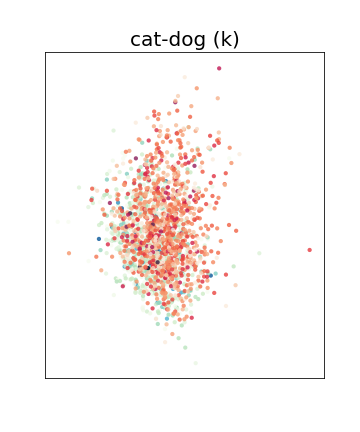}
\includegraphics[width=0.24\linewidth]{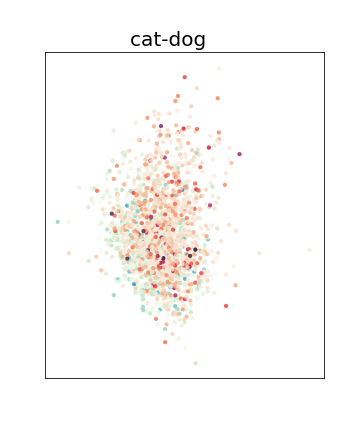}

\vspace{-0.5cm}

\includegraphics[width=0.24\linewidth]{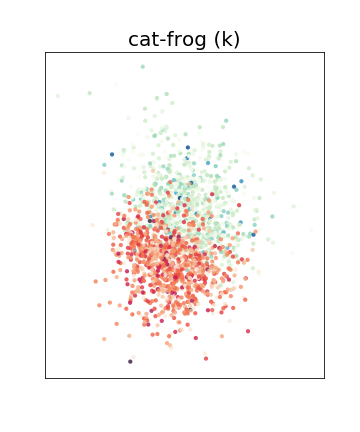}
\includegraphics[width=0.24\linewidth]{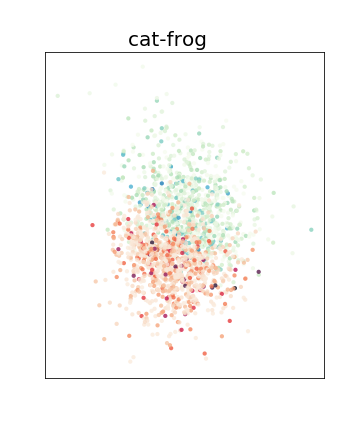}
\includegraphics[width=0.24\linewidth]{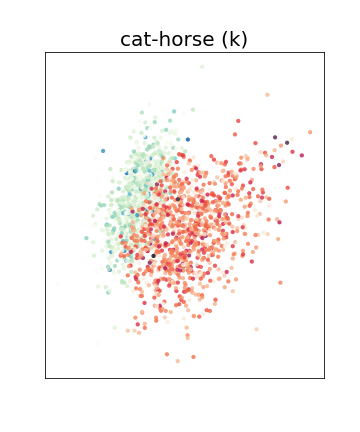}
\includegraphics[width=0.24\linewidth]{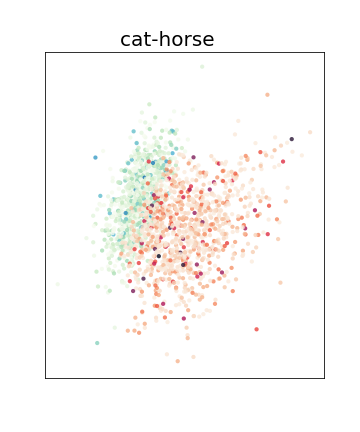}

\vspace{-0.5cm}

\includegraphics[width=0.24\linewidth]{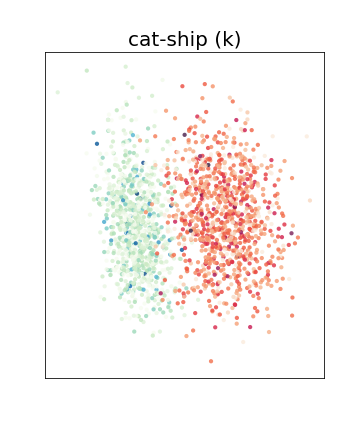}
\includegraphics[width=0.24\linewidth]{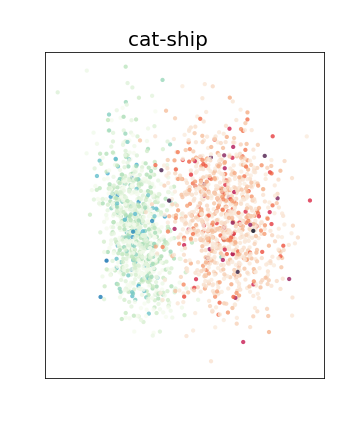}
\includegraphics[width=0.24\linewidth]{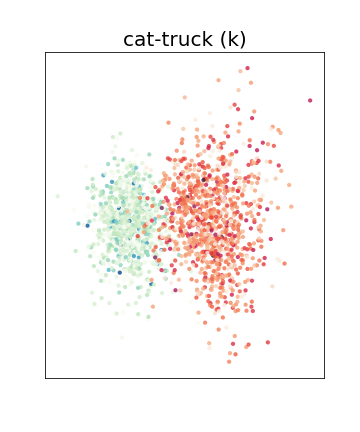}
\includegraphics[width=0.24\linewidth]{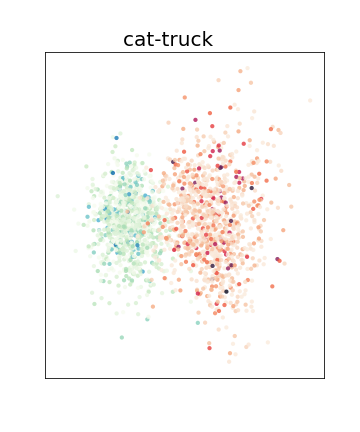}

\vspace{-0.5cm}

\includegraphics[width=0.24\linewidth]{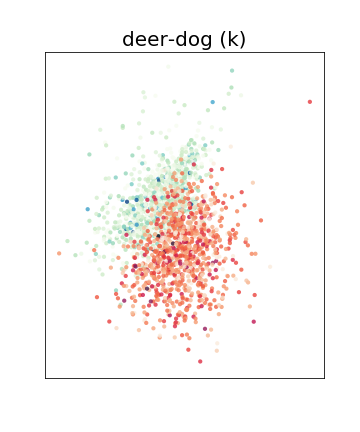}
\includegraphics[width=0.24\linewidth]{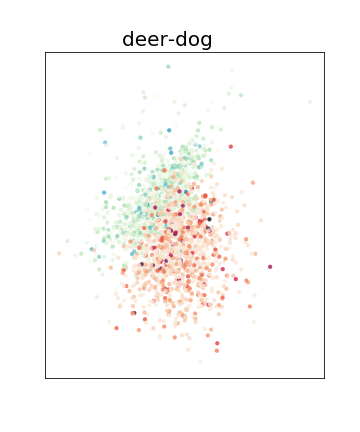}
\includegraphics[width=0.24\linewidth]{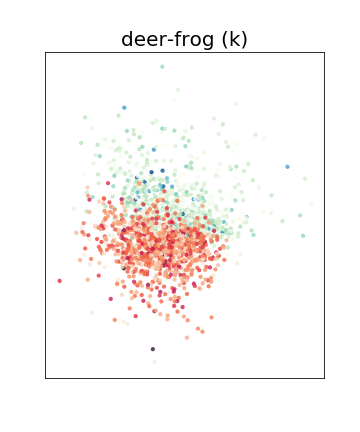}
\includegraphics[width=0.24\linewidth]{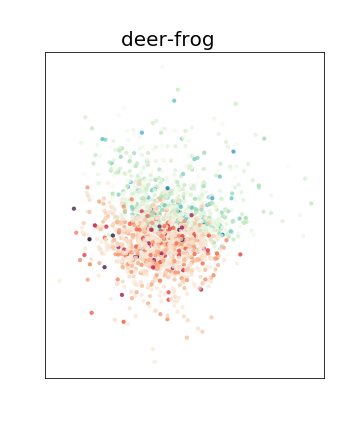}

\vspace{-0.5cm}

\includegraphics[width=0.24\linewidth]{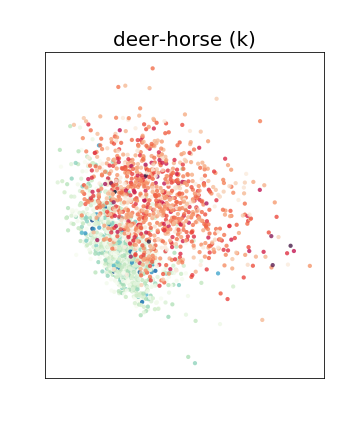}
\includegraphics[width=0.24\linewidth]{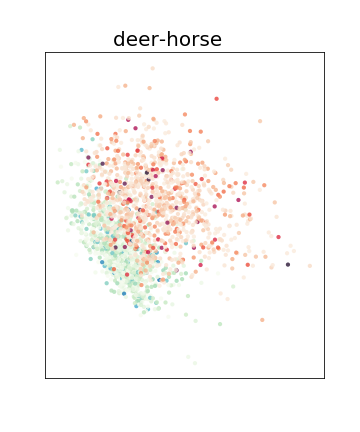}
\includegraphics[width=0.24\linewidth]{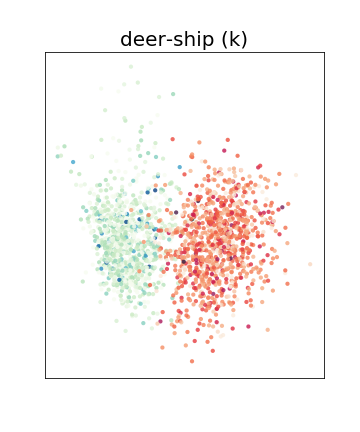}
\includegraphics[width=0.24\linewidth]{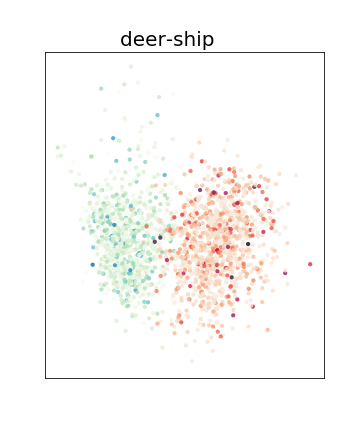}
\caption{\textbf{Part C} 2-d visualizations of the model’s output distribution on CIFAR-10 dataset.}
\end{figure}

%%%%%

\begin{figure}
\includegraphics[trim={0 0.25cm 0 0},clip,width=0.24\textwidth]{figures/pair-plots/scale.png}
\includegraphics[width=0.24\textwidth]{figures/pair-plots-w/scale.png}
\includegraphics[trim={0 0.25cm 0 0},clip,width=0.24\textwidth]{figures/pair-plots/scale.png}
\includegraphics[width=0.24\textwidth]{figures/pair-plots-w/scale.png}

\includegraphics[width=0.24\linewidth]{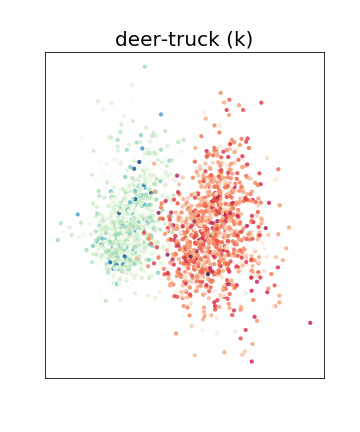}
\includegraphics[width=0.24\linewidth]{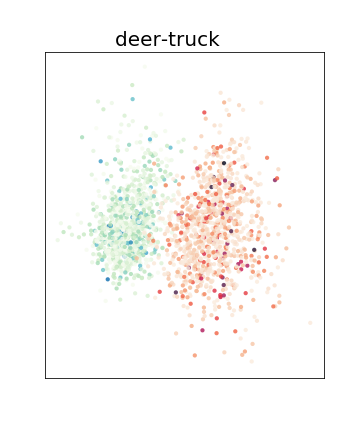}
\includegraphics[width=0.24\linewidth]{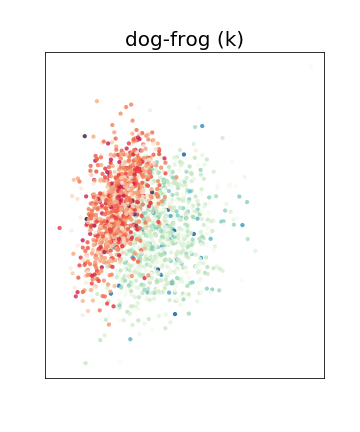}
\includegraphics[width=0.24\linewidth]{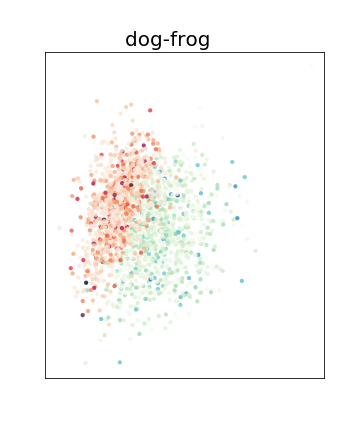}

\vspace{-0.5cm}

\includegraphics[width=0.24\linewidth]{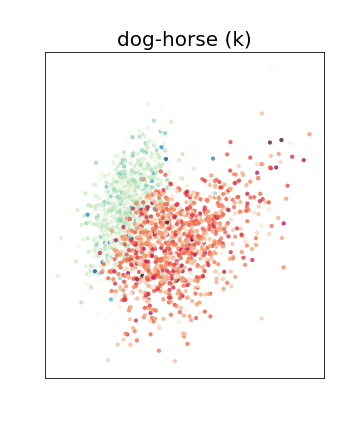}
\includegraphics[width=0.24\linewidth]{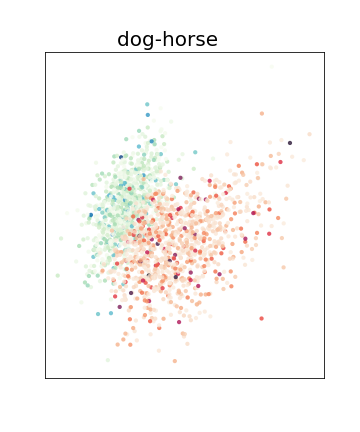}
\includegraphics[width=0.24\linewidth]{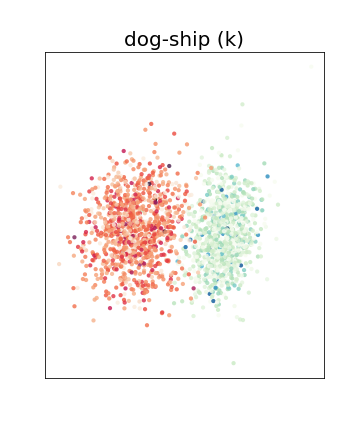}
\includegraphics[width=0.24\linewidth]{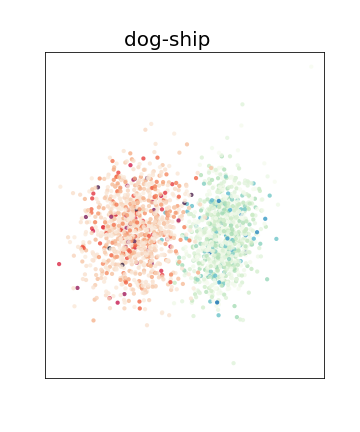}

\vspace{-0.5cm}

\includegraphics[width=0.24\linewidth]{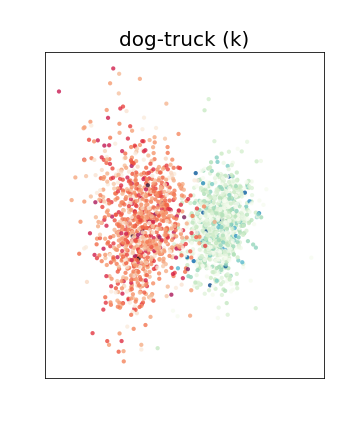}
\includegraphics[width=0.24\linewidth]{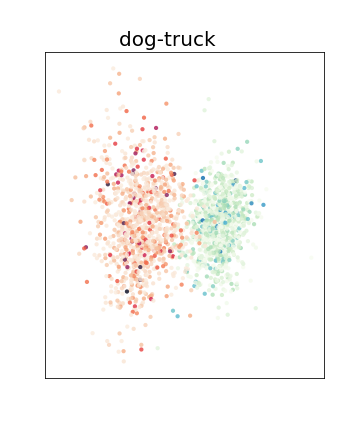}
\includegraphics[width=0.24\linewidth]{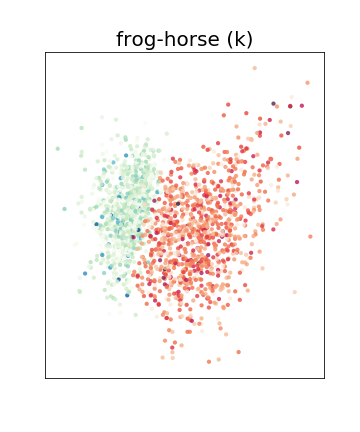}
\includegraphics[width=0.24\linewidth]{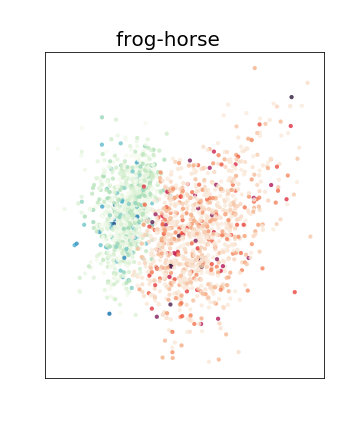}

\vspace{-0.5cm}

\includegraphics[width=0.24\linewidth]{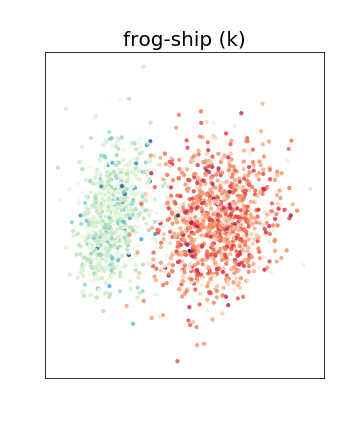}
\includegraphics[width=0.24\linewidth]{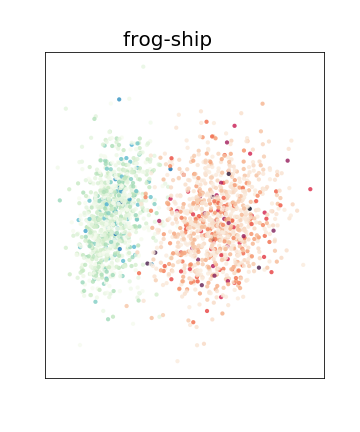}
\includegraphics[width=0.24\linewidth]{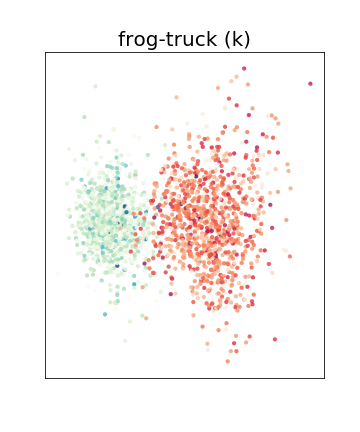}
\includegraphics[width=0.24\linewidth]{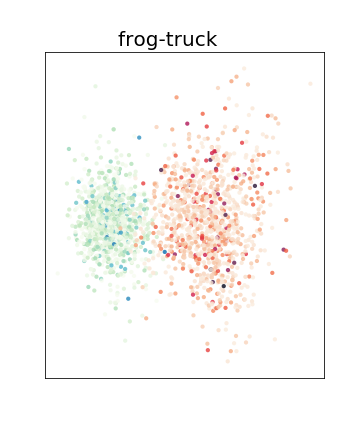}

\vspace{-0.5cm}

\includegraphics[width=0.24\linewidth]{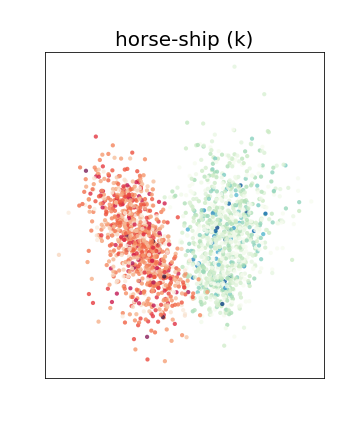}
\includegraphics[width=0.24\linewidth]{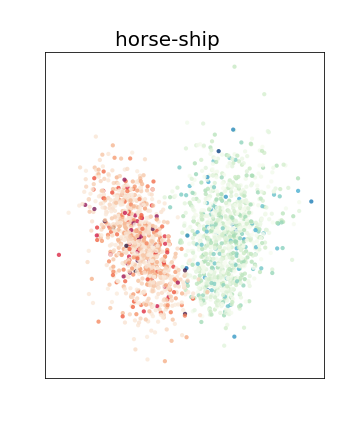}
\includegraphics[width=0.24\linewidth]{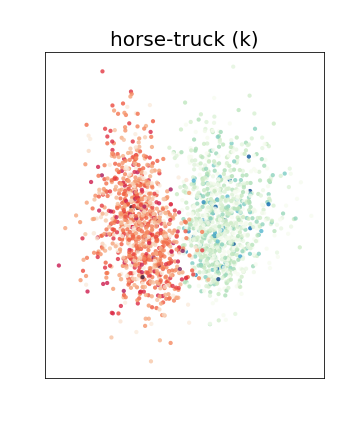}
\includegraphics[width=0.24\linewidth]{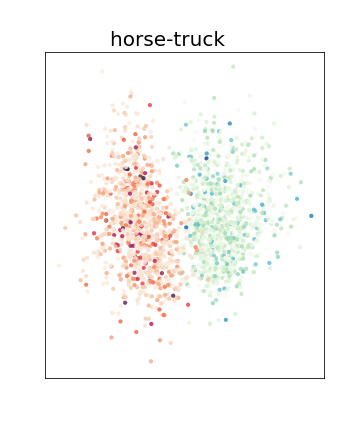}

\vspace{-0.5cm}

\includegraphics[width=0.24\linewidth]{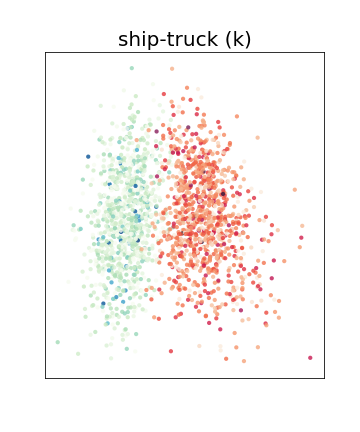}
\includegraphics[width=0.24\linewidth]{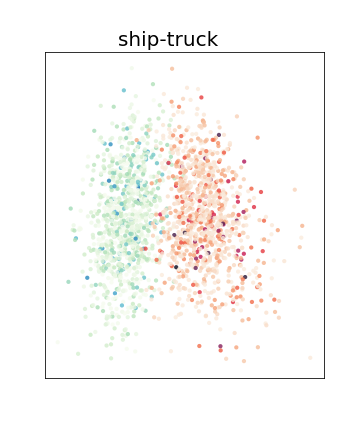}
\caption{\textbf{Part D} 2-d visualizations of the model’s output distribution on CIFAR-10 dataset.}
\end{figure}

%\input{figures/pair-plots/pair-plot}
%\input{figures/pair-plots-w/pair-plot}

%\subsubsection{Different learning rate schedules}

%\subsubsection{Adaptive Attack}
